# Supplementary material for: Rethinking the Variational Interpretation of Nesterov's Accelerated Method
Source: arXiv:2107.05040 source file (2021-07-11)
Supplement: Supplementary file 1 [file appendix.tex]

\newpage

\setcounter{section}{0}
\begin{center}
	\textbf{\Large{Appendix: Proofs and Supplementaries}}
\end{center}

\section{Proofs in Sec.}

\section{}
